# Supplementary material for: Zero-guidance Segmentation Using Zero Segment Labels
Source: arXiv:2303.13396 source file (2023-09-05)
Supplement: Supplementary file 1 [file _supplementary.tex]

\input{_constants}
\review % \review OR \cameraready

\documentclass[10pt,twocolumn,letterpaper]{article}
\input{cvpr_header}
\myexternaldocument{_main}

\usepackage{paralist}

\begin{document}
%% TITLE
\title{Appendix: \paperTitle}
\author{\authorBlock}
\maketitle

\input{12_appendix}
\clearpage
{\small
\bibliographystyle{ieee_fullname}
\bibliography{11_references}
}

\end{document}
